# Supplementary material for: The Pandora's Box Problem with Sequential Inspections
Source: arXiv:2507.07508 source file (2026-04-02)
Supplement: Supplementary file 1 [file appendix_online_problem.tex]

\section{The Online Problem} \label{app:online}

In this section, we consider an \textit{online} variant of our generalized Pandora's box problem in which an adversary presents boxes to Pandora who, in turn, must decide about opening and selecting the particular box, and in which proceeding to the next box (without selecting the current one) results in discarding the current box.
We assume that Pandora does not know the order picked by the adversary (and therefore the problem cannot be solved using backward induction).
In this online setting, the performance of a policy is often  measured by the competitive ratio $\beta$, that is, by a guarantee that regardless of the order in which boxes are presented, her expected performance will be at least $\beta$ of the \textit{offline} optimum expected profit (we refer to our original Pandora's box problem with sequential inspection as the offline problem).

\textit{Main result.}
We show that the class of committing policies defined for the offline problem  can be modified to develop provably good  policies for the online problem. Specifically, we establish that any $\alpha$-approximate committing policy in the offline setting can be converted into an $({\alpha}/{2})$-competitive policy in the online setting.
Therefore, applying our online algorithm to Theorem~\ref{thm:1-1/e} is guaranteed to be $1/2 \cdot\left(1-1/e\right)$-competitive in the online generalized Pandora's box problem. This further suggests that the thresholds capture pivotal characteristics of the problem that guide inspection decisions, even when under incomplete information about the boxes.

\textit{The online problem.}
We consider an online variant of our offline optimization problem where, similarly to the offline problem, all problem parameters are known in advance. That is, boxes are associated with known probability distributions of their prizes and types, and the costs for fully and partially opening boxes are known as well.
However, contrary to the offline problem, in the online setting, Pandora has no control over the order in which boxes are presented.
When a box is presented, she must decide between either selecting the box (after fully and maybe partially opening it) or abandoning the box (either before or after certain opening actions take place).
That is, after box $i$ is presented to Pandora, she has to choose between three courses of action:
\begin{enumerate}
\item Immediately discard the box.
\item Pay $c_i^F$ to F-open the box and observe the realization $v_i$ of its prize $V_i$.
She may then select the box or discard it.
\item Pay $c^P_i$ to P-open the box and observe the realization $t_i$ of its type $T_i$.
Next, she may either discard the box, or pay $c^F_i$ to F-open it and observe the realization $v_i$ of its prize $V_i$.
% \Ali{Is it $v_i$ or $V_i$? Pick one to be consistent. Same below}
In the latter case, she may then either select the box or discard it.
\end{enumerate}

A key feature of this setting is that abandoning a box is irrevocable, meaning that the box in question cannot be subsequently selected.

Technically, the online problem is
a generalization of the model studied by
\cite{esfandiari2019online}, who  first considered the online variant of the standard Pandora's box problem.
They develop an online algorithm that attains a competitive ratio of $1/2$ against the maximum expected profit that can be achieved in the offline variant of the Pandora's box problem (clearly, the offline problem provides an upper bound on the expected profit achievable in the online setting, since Pandora  decides on the ordering of the inspections and may select a box opened earlier).
This worst-case competitive ratio is shown to be tight, making it a natural benchmark to consider.\footnote{Simple counter-arguments show that the performance of any online algorithm against a ``full-information'' benchmark, in which all the realizations of the random parameters are known, can be arbitrarily bad.}

\textit{The online committing policy.}
For every given committing policy $\pi^{F,P}$, we construct a corresponding online policy $\pi^{F,P}_{\textrm{online}}$ as described by Algorithm~\ref{alg:good_online}.
Our algorithm first computes $\tau$---the median profit of the committing policy.
The online policy utilizes the parameter $\tau$ as follows: When presented with a box $i$, if $i\in F$ and $\sigma_i^{F} > \tau$, then  the box is F-opened; it is further selected if $V_i>\tau$, and otherwise, it is discarded.
Alternatively, if $i \in P$ and $\sigma_i^{P}> \tau$, the box is P-opened.
If the conditional F-threshold satisfies $\sigma_i^{F \mid T_i}>\tau$, the box is further F-opened.
Finally, if the realized value satisfies $V_i > \tau$, the box is selected. In all other cases, the box is discarded. %\Ali{To be consistent: Discarded or abandoned?}
 \begin{algorithm}[htbp]
 \footnotesize
  \caption{The competitive algorithm $\pi_{\textrm{online}}^{F,P}$ for the online problem.} \label{alg:good_online}
  \begin{algorithmic}[1]
  % \State Initialize state $(U, P, y) \gets ([N], \emptyset, 0)$
\While { no box has been selected yet and box $i$ is presented }
% \State Sample a $\mathbb{Z}_i$;
\If{$i \in F $ and $\sigma_i^F > \tau$}
        \State F-open box $i$;
        \If{$V_i > \tau$}
            \State Select box $i$;
        \EndIf
\ElsIf{ $i \in P  $ and $\sigma_i^P > \tau$}
        \State P-open box $i$;
        \If{$\sigma_i^{F \mid T_i} > \tau$}
            \State F-open box $i$;
            \If{$V_i > \tau $}
                \State Select box $i$;
            \EndIf
        \EndIf
\EndIf
\State Skip box $i$;
\EndWhile
  \end{algorithmic}
\end{algorithm}

Let $\textrm{OPT}_{\textrm{off}}$ denote the expected profit of an optimal policy in the offline variant of our generalized Pandora's box problem
(where boxes may be revisited). Our main result can be stated as follows.

\begin{theorem} \label{thm:online_const_committing}

Let $\pi^{F,P}$ be an $\alpha$-approximation committing policy for the offline problem. Let $K_{m} =  \underset{}{\max}  \left\{  \underset{i \in F}{\max}\left\{ K_i \right\} , \underset{i \in P}{\max}   \left\{ \widetilde{K}_i\right\} \right\}$, and set $\tau$ to the median of $K_{m}$, that is, $\operatorname{Pr} \left[ K_{m}  > \tau   \right] = 1/2$. \footnote{For simplicity, we assume  for any $\epsilon > 0$, there exists $\delta > 0 $ such that $\operatorname{Pr} \left[ \tau - \delta < K_{m} < \tau + \delta   \right] < \epsilon$. }   For the online problem, policy $\pi_{\textrm{online}}^{F,P}$ generates an expected profit of at least $\frac{1}{2} \alpha \cdot \mathrm{OPT}_{\mathrm{off}}$ for any presented sequence.

\end{theorem}

Theorem~\ref{thm:online_const_committing} provides a theoretical  guarantee for our method, allowing us to convert any committing policy into an online policy with only a constant-factor loss of optimality (e.g., the policies defined in Theorems~\ref{thm:simple_constant_apx} and \ref{thm:1-1/e}). The proof of this theorem is deferred to Appendix~\ref{appendix:thm_online_const_committing}. 

We next show that under a certain assumption, the same guarantee holds for the optimal policy (rather than a committing policy). First, denote $K_{\max} =   \max \left\{ \underset{i \in [N]}{\max} \{  K_i\}   , \underset{i \in [N]}{\max}  \{ \widetilde{K}_i \}  \right\} $ (which clearly satisfies $K_{\max}\geq K_{m}$).

\begin{assumption} \label{assumption:online_large_tau} The median of the maximal profit $K_{\max}$ exceeds the F-threshold of all boxes for which $\sigma_i^P\geq\sigma_i^F$, that is,
$$
\tau > \max_{i : \sigma_i^P \geq \sigma_i^F } \left\{ \sigma_i^F \right\}.
$$
\end{assumption}
Intuitively, this assumption captures problem instances where the median is large compared with the thresholds. For example, this might occur when there is a relatively large number of boxes and  relatively small number of box ``classes'', in which case, the median approaches the maximal value in the probability distributions' supports. For example, in the context of job recruiting, there could be a small number of candidates' profiles, but a relatively large pool of candidates.

\begin{corollary} \label{cor:online_optimal_under_assumption}
Given a problem instance $\left\{c_i^F,c_i^P, \mathcal{D}_i \right\}_{i=1}^{N}$,
let $\tau$ be such that $\operatorname{Pr}\left[ K_{\max} > \tau \right] = 1/2 $. \footnote{For simplicity, we once again assume that for any $\epsilon > 0$, there exists $\delta > 0 $ such that $\operatorname{Pr} \left[ \tau - \delta < K_{\max} < \tau + \delta   \right] < \epsilon$. }
We define the committing policy $\pi^{F,P}$ using $P=\{i \in [N] \mid \sigma_i^P > \tau \geq \sigma_i^F \}$ and $F = [N] / P$.
Under Assumption~\ref{assumption:online_large_tau},  policy $\pi^{F,P}_{\textrm{online}}$ generates an expected profit of at least $1/2 \cdot \mathrm{OPT}_{\mathrm{off}}$.
Moreover, under this assumption, there is no online policy that  guarantees a constant-factor competitive ratio strictly greater than $1/2$.
\end{corollary}
The proof of Corollary~\ref{cor:online_optimal_under_assumption} is deferred to Appendix~\ref{appendix:cor_online_optimal_under_assumption}. overall, our analysis shows that committing policies can be resilient in circumstances where there is uncertainty about the availability of boxes.

\subsection{Proof of Theorem~\ref{thm:online_const_committing}}
\label{appendix:thm_online_const_committing}
We let $u_{\textrm{online}} \left( \pi_{\textrm{online}}^{F,P} \right) $ be expected profit of the online policy $\pi_{\textrm{online} }^{F,P}$. 
The proof proceeds in two main steps.
First, we construct an upper bound on  $\textrm{OPT}_{\textrm{off}}$ that depends on $\tau$.
Then, we use this quantity to to lower bound $u_{\textrm{online}} \left( \pi_{\textrm{online}}^{F,P} \right) $ up to a constant multiplicative factor.

When box $i$ is presented to Pandora, let $\nu_i(\tau)$ be the bonus she can get above $\tau$. We have the following two lemmas. 
\begin{lemma} \label{lemma:online_proof_1}
The expected bonus she can get above $\tau$ is 
\begin{equation}  \label{eq:online_expected_reward_surpassing}
  \mathbb{E}\left[ \nu_i(\tau) \right] = \mathbbm{1}\left\{ i \in F \right\}  \cdot \mathbb{E} \left[   \left(    K_i   -\tau  \right)^+   \right] + \mathbbm{1} \left\{ i \in P \right\}  \cdot \mathbb{E} \left[   \left( \widetilde{K_i}-\tau  \right)^+ \right]  \  .  
\end{equation}
Moreover, given an $\alpha$-approximation committing policy $\pi^{F,P}$ for the offline problem,  we have 
\begin{equation} \label{eq:online_upper_bound_offline}
    \alpha \cdot \textrm{OPT}_{\textrm{off}} \leq \tau +   \sum_{i=1}^{N} \mathbb{E} \left[ \nu_i(\tau) \right] \ . 
\end{equation}
\end{lemma}

\begin{lemma} \label{lemma:online_proof_2}
$u_{\textrm{online}} \left( \pi_{\textrm{online}}^{F,P} \right) \geq \frac{1}{2} \tau + \frac{1}{2}  \sum_{i=1}^{N} \mathbb{E} \left[ \nu_i(\tau) \right]$.
\end{lemma}

Combining Lemma~\ref{lemma:online_proof_1} and~\ref{lemma:online_proof_1} together yields that 
$$
u_{\textrm{online}} \left( \pi_{\textrm{online}}^{F,P} \right) \geq \frac{1}{2} \alpha  \cdot \textrm{OPT}_{\textrm{off}} \ ,
$$
which is desired. The rest of this proof is to show the preceding two lemmas.

\begin{myproof2}{Lemma \ref{lemma:online_proof_1}}
First, since $\pi^{F,P}$ is an $\alpha$-approximation algorithm for the offline problem, we have
\begin{eqnarray}
   \alpha \cdot \textrm{OPT}_{\textrm{off}}  &\leq&  u_{\rm{I}}\left( \pi^{F,P} \right)    \nonumber \\
   &=&  \mathbb{E}\left[ \max \left\{ \underset{i \in F}{\max} \{  K_i\}   , \underset{i \in P}{\max}  \{ \widetilde{K}_i \}  \right\}\right] \label{eq:online_alpha_committing_upper_bound_1}       \\
   &=& \tau + \mathbb{E}\left[ \max \left\{ \underset{i \in F}{\max}  \{  K_i  - \tau \}   , \underset{i \in P}{\max}  \{ \widetilde{K}_i - \tau \}   \right\}\right]          \nonumber \\
   &\leq& \tau + \mathbb{E}\left[ \max \left\{ \underset{i \in F}{\max}  \{  \left( K_i  - \tau\right)^+ \}   , \underset{i \in P}{\max}  \{  \left( \widetilde{K}_i - \tau \right)^+ \}   \right\}\right]    \nonumber       \\
   &\leq&  \tau +  \mathbb{E}\left[ \sum_{i \in F }    \left( K_i  - \tau\right)^+    +  \sum_{i \in P}  \left( \widetilde{K}_i - \tau \right)^+  \right]  \ ,  \label{eq:lemma:online_proof_1_1}  
\end{eqnarray}
where equation~\eqref{eq:online_alpha_committing_upper_bound_1} follows from Lemma~\ref{lemma:committing} with respect to the committing policy $\pi^{F,P}$.
Equation~\eqref{eq:lemma:online_proof_1_1} decomposes the expected profit into two components: the median $\tau$ and the expected bonus above $\tau$, which we denote by $\mathbb{E} \left [\nu_i(\tau) \right]$. 
% Note that the policy  $\pi_{\textrm{online}}^{F,P}$ never selects a prize lower than $\tau$. 

Assume that box $i$ is presented and $i \in F$. Then, policy $\pi_{\textrm{online}}^{F,P}$ will F-open box $i$ and select it if $V_i > \tau$. 
Therefore, the expected bonus above $\tau$ is  
\begin{eqnarray}
   \mathbb{E}\left[ \nu_i(\tau) \right] &=& -c_i^F + \operatorname{Pr}\left[ V_i > \sigma_i^F \right] \left( \mathbb{E}\left[V_i  \mid V_i > \sigma_i^F \right] - \tau \right) +  \operatorname{Pr}\left[ \tau < V_i \leq \sigma_i^F  \right] \left( \mathbb{E} \left[ V_i \mid \tau < V_i \leq \sigma_i^F  \right] - \tau \right)   \nonumber  \\
   &=& \operatorname{Pr}\left[ V_i > \sigma_i^F \right] \left( \sigma_i^F - \tau \right) +  \operatorname{Pr}\left[ \tau < V_i \leq \sigma_i^F  \right] \left( \mathbb{E} \left[ V_i \mid \tau < V_i \leq \sigma_i^F  \right] - \tau \right) + \operatorname{Pr}\left[V_i \leq  \tau  \right] \cdot 0 \nonumber  \\
   &=& \mathbb{E}\left[  \left(  \min \left \{ V_i, \sigma_i^F \right \}  - \tau   \right)^+ \right]  = \mathbb{E}\left[  \left(  K_i - \tau   \right)^+ \right] \ .  \nonumber 
\end{eqnarray}

Similarly, given that a box $i$ is presented and $i \in P $, the expected bonus above $\tau$ is 
\begin{eqnarray}
   \mathbb{E}\left[ \nu_i(\tau) \right]  &=&  -c_i^P +  \sum_{t_i: \sigma_i^{F \mid t_i} > \sigma_i^P } \operatorname{Pr} \left[ T_i=t_i \right] \Bigg( -c_i^F + \operatorname{Pr} \left[ V_i > \sigma_i^P \mid T_i=t_i \right] \left(  \mathbb{E}\left[ V_i \mid  V_i > \sigma_i^P, T_i=t_i \right] -\tau \right)   \nonumber   \\
  & &   +  \operatorname{Pr} \left[ \tau < V_i \leq \sigma_i^P \mid  T_i = t_i  \right]  \left( \mathbb{E} \left[ V_i \mid  \tau < V_i \leq \sigma_i^P, T_i=t_i \right]- \tau  \right)   \Bigg)           \nonumber  \\
   & & +  \sum_{t_i:  \tau < \sigma_i^{F \mid t_i} \leq \sigma_i^P } \operatorname{Pr} \left[ T_i=t_i \right]     \Bigg( -c_i^F + \operatorname{Pr} \left[ V_i > \sigma_i^{F \mid t_i} \mid T_i=t_i \right] \left(  \mathbb{E}\left[ V_i \mid  V_i > \sigma_i^{F \mid t_i}, T_i=t_i \right] -\tau \right)   \nonumber   \\
  & &   +  \operatorname{Pr} \left[ \tau < V_i \leq \sigma_i^{F \mid t_i} \mid  T_i = t_i  \right]  \left( \mathbb{E} \left[ V_i \mid  \tau < V_i \leq \sigma_i^{F \mid t_i} , T_i=t_i \right]- \tau  \right)   \Bigg)            \nonumber   \\
  &=&  \sum_{t_i: \sigma_i^{F \mid t_i} > \sigma_i^P } \operatorname{Pr} \left[ T_i=t_i \right] \Bigg(  \operatorname{Pr} \left[ V_i > \sigma_i^P \mid T_i=t_i \right] \left( \sigma_i^P - \tau \right)   \nonumber   \\
  & &   +  \operatorname{Pr} \left[ \tau < V_i \leq \sigma_i^P \mid  T_i = t_i  \right]  \left( \mathbb{E} \left[ V_i \mid  \tau < V_i \leq \sigma_i^P, T_i=t_i \right]- \tau  \right)   \Bigg)            \nonumber  \\
   & & +  \sum_{t_i:  \tau < \sigma_i^{F \mid t_i} \leq \sigma_i^P } \operatorname{Pr} \left[ T_i=t_i \right]     \Bigg( \operatorname{Pr} \left[ V_i > \sigma_i^{F \mid t_i} \mid T_i=t_i \right]   \left( \sigma_i^{F \mid t_i} - \tau  \right)     \nonumber   \\
  & &   +  \operatorname{Pr} \left[ \tau < V_i \leq \sigma_i^{F \mid t_i} \mid  T_i = t_i  \right]  \left( \mathbb{E} \left[ V_i \mid  \tau < V_i \leq \sigma_i^{F \mid t_i} , T_i=t_i \right]- \tau  \right)   \Bigg)            \nonumber   \\
  &=&   \mathbb{E}\left[  \left(  \min \left \{ V_i, \sigma_i^{F \mid t_i} , \sigma_i^P \right \}  - \tau   \right)^+ \right] = \mathbb{E}\left[  \left(  \widetilde{K_i} - \tau   \right)^+ \right] \ .   \nonumber 
\end{eqnarray}
We conclude that
$$
 \mathbb{E}\left[ \nu_i(\tau) \right] = \mathbbm{1}\left\{ i \in F \right\}  \cdot \mathbb{E} \left[   \left(    K_i   -\tau  \right)^+   \right] + \mathbbm{1} \left\{ i \in P \right\}  \cdot \mathbb{E} \left[   \left( \widetilde{K_i}-\tau  \right)^+ \right]  \  .  
$$
\end{myproof2}

\begin{myproof2}{Lemma \ref{lemma:online_proof_2}}

First, we introduce some notations. 
We denote by $\omega$ any sequence of boxes chosen by the adversary, where  $\omega(i)$ denotes the rank of box $i$ in the sequence (e.g., $\omega(i)=1$ indicates that box $i$ is presented in the $1^{\text{st}}$ position). 
We denote by $\zeta(\omega)$ the probability that the adversary chooses the sequence $\omega$. We denote by $\phi(i; \omega)$ the probability that boxes before box $i$ are all passed conditional on that the sequence $\omega$ is given. 

By construction of the policy $\pi_{\textrm{online}}^{F,P}$, we observe that it selects the first box $i$ that satisfies
$$  \mathbbm{1} \left\{ i \in F \right\}  \cdot       K_i   +    \mathbbm{1} \left\{ i \in P \right\}    \cdot \widetilde{K_i}   > \tau \ .$$
Therefore, the policy will get $\tau$ as long as $K_m > \tau$ (recall $K_m $ is defined as $K_{m} =  \underset{}{\max}  \left\{  \underset{i \in F}{\max}\left\{ K_i \right\} , \underset{i \in P}{\max}   \left\{ \widetilde{K}_i\right\} \right\}$). Note that the total expected profit can be decomposed to the quantity $\tau$ and the bonus above $\tau$, and thus, we have 
\begin{eqnarray}
u_{\textrm{online}} \left( \pi_{\textrm{online}}^{F,P} \right)   &\geq&  \operatorname{Pr} \left[K_{m} > \tau \right] \cdot \tau  +  \sum_{\omega}  \Bigg( \zeta(\omega) \sum_{i=1}^{N} \phi(i; \omega)  \cdot \mathbb{E} \left[ \nu_i(\tau) \mid  \text{boxes before } i  \text{ are skipped given  } \omega \right]  \Bigg)  \nonumber \\ 
&=& \operatorname{Pr} \left[K_{m} > \tau \right] \cdot \tau  +  \sum_{\omega}  \left( \zeta(\omega) \sum_{i=1}^{N} \phi(i; \omega)  \cdot \mathbb{E} \left[ \nu_i(\tau) \right]  \right) \ , \label{eq:online_u_1}
\end{eqnarray}
where equation~\eqref{eq:online_u_1} follows from the mutual independence of boxes.  
Let $q_j$ be the probability that a presented box $j$ is not selected, that is,
$$
q_j = \operatorname{Pr} \left[ \mathbbm{1} \left\{ j \in F \right\}  \cdot       K_j   +    \mathbbm{1} \left\{ j \in P \right\}    \cdot \widetilde{K_j} \leq \tau \right] \ .
$$
Hence, the probability $\phi(i; \omega) $ can be expressed as 
\begin{eqnarray}
\phi(i; \omega)  &=& \underset{j: \omega(j) < \omega(i)}{\bigwedge} \left\{ \mathbbm{1} \left\{ j \in F \right\}  \cdot       K_j   +    \mathbbm{1} \left\{ j \in P \right\}   \cdot \widetilde{K_j} \leq \tau \right\}  \nonumber \\ 
&=&  \prod_{j: \omega(j) < \omega(i) } q_j  \label{eq:online_phi_q}  \ . 
\end{eqnarray}
Equation~\eqref{eq:online_phi_q} follows from the mutual independence of boxes. Combining inequality~\eqref{eq:online_u_1} and equation~\eqref{eq:online_phi_q} yields that 
\begin{eqnarray}
u_{\textrm{online}} \left( \pi_{\textrm{online}}^{F,P} \right)   &\geq& \operatorname{Pr} \left[K_{m} > \tau \right] \cdot \tau  +  \sum_{\omega} \zeta(\omega) \sum_{i=1}^{N} \prod_{j: \omega(j) < \omega(i) } q_j   \cdot \mathbb{E} \left[ \nu_i(\tau) \right]  \nonumber \\ 
&=& \operatorname{Pr} \left[K_{m} > \tau \right] \cdot \tau  + \sum_{i=1}^{N}  \sum_{\omega} \zeta(\omega)  \prod_{j: \omega(j) < \omega(i) } q_j   \cdot \mathbb{E} \left[ \nu_i(\tau) \right]   \nonumber \\ 
&\geq& \operatorname{Pr} \left[K_{m} > \tau \right] \cdot \tau  + \sum_{i=1}^{N}   \prod_{j \neq i } q_j   \cdot \mathbb{E} \left[ \nu_i(\tau) \right]  \label{eq:online_u_2}  \nonumber \\ 
&\geq&  \operatorname{Pr} \left[K_{m} > \tau \right] \cdot \tau  + \prod_{i=1}^{N} q_j   \cdot \sum_{i=1}^{N}   \mathbb{E} \left[ \nu_i(\tau) \right]  \nonumber \\ 
&=& \operatorname{Pr} \left[K_{m} > \tau \right] \cdot \tau  +   \operatorname{Pr} \left[K_{m} \leq \tau \right] \sum_{i=1}^{N}   \mathbb{E} \left[ \nu_i(\tau) \right]   \label{eq:online_u_3}  \nonumber \\ 
&=& \frac{1}{2} \tau  +   \frac{1}{2} \sum_{i=1}^{N}   \mathbb{E} \left[ \nu_i(\tau) \right]   \ .  \label{eq:online_u_4}
\end{eqnarray}
% Inequality~\ref{eq:online_u_2} simply follows from the fact that 

\end{myproof2}

\subsection{Proof of Corollary~\ref{cor:online_optimal_under_assumption}}
\label{appendix:cor_online_optimal_under_assumption}

First, we give an upper bound on $\mathrm{OPT}_{\mathrm{off}}$:
\begin{eqnarray}
 \textrm{OPT}_{\text{off}} &\leq& \max_{\pi \in \Pi}~ u_{\rm{II}}\left( \pi \right)  \nonumber  \\
   &\leq&  \mathbb{E}\left[ \max \left\{ \underset{i \in [N]}{\max} \{  K_i\}   , \underset{i \in [N]}{\max}  \{ \widetilde{K}_i \}  \right\}  \right]  \nonumber \\
   &=& \tau + \mathbb{E}\left[ \underset{i \in [N]}{\max} \left\{   \max \left\{   K_i   ,  \widetilde{K}_i \right\}  - \tau   \right\}\right]          \nonumber \\
   &\leq&  \tau + \mathbb{E}\left[ \underset{i \in [N]}{\max} \left\{ \left(   \max \left\{   K_i   ,  \widetilde{K}_i \right\}  - \tau   \right)^+  \right\}   \right]          \nonumber   \\
   &\leq&  \tau + \mathbb{E}\left[ \sum_{i=1}^{N } \left(   \max \left\{   K_i   ,  \widetilde{K}_i \right\}  - \tau   \right)^+  \right]          \nonumber   \\
   &=&   \tau+\sum_{i=1}^{N} \Bigg [ \underbrace{\mathbb{E}\left[  \left(\max \left\{K_{i}, \widetilde{K}_{i}\right\} -\tau\right)^{+} \mid \sigma_i^P \leq \tau, \sigma_i^F \leq \tau \right] }_{=0} \mathbbm{1} \left\{ \sigma_i^P \leq \tau, \sigma_i^F \leq \tau  \right\}             \nonumber    \\
       &+&   \mathbb{E}\left[\Big(K_{i} -\tau\Big)^{+} \mid  \sigma_i^P \leq \tau, \sigma_i^F > \tau \right] \mathbbm{1} \left\{ \sigma_i^P \leq \tau, \sigma_i^F > \tau  \right\}        \nonumber \\
       &+&   \mathbb{E}\left[\left(\widetilde{K}_{i} -\tau\right)^{+} \mid  \sigma_i^P > \tau, \sigma_i^F \leq \tau \right] \mathbbm{1} \left\{ \sigma_i^P > \tau, \sigma_i^F \leq \tau  \right\}         \nonumber \\
       &+&   \mathbb{E}\left[\Big(K_{i} -\tau \Big)^{+} \mid  \sigma_i^P > \tau, \sigma_i^F > \tau , \sigma_i^F > \sigma_i^P \right] \mathbbm{1} \left\{ \sigma_i^P > \tau, \sigma_i^F > \tau, \sigma_i^F > \sigma_i^P  \right\}                \nonumber \\
       &+&       \mathbb{E}\left[\left(\max \left\{K_{i}, \widetilde{K}_{i}\right\} -\tau\right)^{+} \mid  \sigma_i^P > \tau, \sigma_i^F > \tau , \sigma_i^P \geq \sigma_i^F \right] \underbrace{\mathbbm{1} \left\{ \sigma_i^P > \tau, \sigma_i^F > \tau,  \sigma_i^P \geq \sigma_i^F  \right\}}_{=0 \text{ by Assumption \ref{assumption:online_large_tau} }}                \Bigg ] \nonumber\\
  %\end{eqnarray}
  %\begin{eqnarray}
   &\leq&  \tau + \sum_{i=1}^{N} \Bigg[ \underbrace{\mathbb{E} \left[ \left( K_i -\tau \right)^+ \mid \sigma_i^P \leq \tau, \sigma_i^F \leq \tau  \right] }_{=0}  \mathbbm{1} \left\{ \sigma_i^P \leq \tau, \sigma_i^F \leq \tau \right\}   \nonumber
      \nonumber \\
      &+& \mathbb{E} \left[ \left( K_i -\tau \right)^+ \mid \sigma_i^P \leq \tau , \sigma_i^F > \tau  \right]   \mathbbm{1} \left\{ \sigma_i^P \leq \tau , \sigma_i^F > \tau \right\}  \nonumber\\
   &+&   \mathbb{E} \left[ \left( \widetilde{K}_i-\tau \right)^+ \mid \sigma_i^P > \tau, \sigma_i^F \leq \tau \right]   \mathbbm{1} \left\{ \sigma_i^P > \tau, \sigma_i^F \leq \tau \right\}   \nonumber \\
        &+& \mathbb{E} \left[ \left( K_i -\tau \right)^+ \mid \sigma_i^P > \tau , \sigma_i^F > \tau \right]   \underbrace{\mathbbm{1} \left\{ \sigma_i^P > \tau , \sigma_i^F > \tau \right\}}_{ \geq \mathbbm{1} \left\{ \sigma_i^P > \tau , \sigma_i^F > \tau , \sigma_i^F>\sigma_i^P \right\} } \Bigg]   \label{eq:online_cor_long_transition_1} \nonumber \\
   &=&   \tau+\sum_{i=1}^{N} \mathbb{E} [\nu_i]      \ .
       \label{eq:online_1/2_1}
\end{eqnarray}
\Jingwei{TODO}
The first inequality is due to Corollary~\ref{cor:free_info_problem}. 
The sequence of inequalities leading up to equation~\eqref{eq:online_cor_long_transition_1} follow from simple arithmetic and using Assumption~\ref{assumption:online_large_tau}.
The last equality follows equation~\eqref{eq:online_expected_reward_surpassing} and the definition of the committing policy $\pi^{F,P}$ where
$P=\{i \in [N] \mid \sigma_i^P > \tau \geq \sigma_i^F \}$ and $F = [N] / P$. 
By rearranging inequality~\eqref{eq:online_1/2_1},  we obtain
$$
\sum_{i=1}^{N} \mathbb{E} [\nu_i] \geq \mathrm{OPT}_{\mathrm{off}} - \tau \ .
$$

Next, policy $\pi^{F,P}$ is a committing policy, and thus, following a derivation similar to that of inequality~\eqref{eq:online_u_4}, we have % similarly to the proof of Theorem~\ref{thm:online_const_committing}, it satisfies:
$$
u_{\textrm{online}} \left( \pi_{\textrm{online}}^{F,P} \right)
\geq
\frac{1}{2} \tau  +  \frac{1}{2} \sum_{i=1}^{N} \mathbb{E} [\nu_i] \ .
$$
By combining the latter inequality with inequality~\ref{eq:online_1/2_1}, we have $u_{\textrm{online}}\left( \pi_{\textrm{online} }^{F,P}\right)  \geq \frac{1}{2} \cdot \mathrm{OPT}_{\mathrm{off}}$.

Finally, to show that the competitive ratio of $1/2$ is tight, we revisit an example used in the context of the prophet inequalities \citep{samuel1984comparison}. Consider a problem instance with two boxes:
\begin{itemize}
    \item Box 1: $c_1^F=0, c_1^P=100, V_1=1$.
    \item Box 2: $c_2^F=0, c_2^P=100$, $V_2 = \frac{1}{\epsilon}$ with probability  $\epsilon $ and $V_2 = 0 $ with probability  $1-\epsilon $.
\iffalse
        \item Box 3: $c_3^F=0.2 \epsilon , c_3^P=0.01 \epsilon $,
    $$
        T_3 = \left\{\begin{array}{ll}
    { A } & {\text{with probability } 0.5 } \\
    {B} & {\text{with probability } 0.5 }
    \end{array}\right., V_3 \mid A = \left\{\begin{array}{ll}
    { \epsilon} & {\text{with probability } 0.2 } \\
    {0} & {\text{with probability } 0.8 }
    \end{array}\right., V_3 \mid B = \left\{\begin{array}{ll}
    {\epsilon } & {\text{with probability } 0.8 } \\
    {0 } & {\text{with probability } 0.2 }
    \end{array} \right.
    .$$
    So $\sigma_3^P > \sigma_3^F$.
\fi
\end{itemize}
In both cases, the F-opening cost is negligible while the P-opening costs is high, making it disadvantageous to P-open any box. The F-thresholds are equal to the largest values in the supports, and thus,  $K_i=V_i$. In addition, we have 
$$
K_{\max} = \left\{\begin{array}{ll}
{1} & {\text{with probability } 1- \epsilon } \\
{\frac{1}{\epsilon}} & {\text{with probability } \epsilon }
\end{array}\right.,
\text{ and }
\mathbb{E} \left[ K_{\max} \right] = 2-\epsilon.
$$
Consider a scenario in which the adversary is presenting box 1 and then box 2. If an online policy selects box 1, its profit is 1, otherwise, if it skips box 1 and F-opens box 2, its expected profit is also 1. Since $\epsilon$ can be arbitrarily small, the best-possible competitive ratio does not exceed $1/2$.
\Halmos
